# Supplementary material for: Heterogeneous Multi-Robot Graph Coverage with Proximity and Movement Constraints
Source: arXiv:2412.10083 source file (2024-12-17)
Supplement: Supplementary file 1 [file rebuttal.tex]

\section{Rebuttal}
We thank all reviewers for going over the paper. Editorial comments will be addressed, we would like to address two key points raised by the reviewers.

6Enh:

Number of Robots: the complexity of our algorithms scales linearly with the size of the graph, but may be exponential in the number of robots.  So, for a large number of robots, computation may be prohibitive.  However, even for a small number of robots, the speed-up can be substantial.  For example, we ran simulations on real-world graphs with hundreds of nodes (e.g. hotel floor plans), and even with 3 robots get a speed-up of 44\%. We will include these findings in the paper.

tKsV:

Thanks for the detailed comments.  We will fix them according to your editorial and structural recommendations.

Real-world instances: We ran our algorithm on real-world instances of hotel floor plans (useful, for example, in a search and rescue setting).  We will include the findings in the paper.

Section 1.1 (2nd bullet):

Problem novelty: both MRCGC and MRFGC are both novel.

Section 5 (2nd bullet):

$|PS(j)|$ independent of $n$: this is formalized in Lemma 4.  The size depends on $k$ and $d$ and $\textsf{tw}$, but not on graph size $n$. The reason is that are determined by the $k$-neighborhood the the bag. Since transitions cannot repeat, a pigeonhole principle argument bounds signature length, independent of $n$.

Section 5.1:

Size of table $j$: In the algorithm, as described, the table size is exactly $|PS(j)|$, except when applying the rules for deletion of rows (detailed after point 3). 

% [Note that making the FPT algorithm practical revolves around reducing the table sizes, which can be done without compromising on traversal time in certain scenarios. For instance, with k=3 connected robots, we show certain transitions types cannot repeat even once, significantly reducing table sizes. However, this is beyond scope of section 5.1.]

Section 6:
1st bullet: It is MRFTC, but only for collpasible formations.
3rd bullet: Algorithm GreedyTraverse.

Gw13:

1. Heterogenicity: Indeed, we use the term "heterogeneous" to mean that the robots may differ in design, capabilities, and functionalities. They may also move independently. They are, however, all managed by a single algorithm.  So, the system is not distributed. Our use of the term follows many others in the literature, e.g. a recent survey [1] that defines: "heterogeneity in a coverage scenario can be defined in different aspects, such as different movement or sensing capabilities of the robots or different platforms". See also [2,3,4] that study heterogeneous robots with a centralized planner. 
Indeed, part of the literature considers heterogeneous systems that are also distributed (also covered in related work), which we do not. We will clarify this point.

2. Tethered Coverage: Thanks for pointing out this related work. We note that tethered coverage may be sub-optimal in our setting, as evidenced by the following examples.  Consider a starfish-shaped graph with 4 arms, each of length $k/4$. The entire graph can be covered with $k$ robots in $k/2$ steps (assuming the robots start and end at the center). With a tethered chain, the number of steps would be double (the exact number depends on the exact definition of a tethered coverage). With $2x$ arms, each of length $k/2x$, the tethered coverage time grows to $x$-fold of the optimal.  By adding more arms, this reasoning can be extended to any number of nodes. Similar behavior can be obtained for other graph structures. 

4. Arrow Symbols - Imagine a tree with the root placed at the top. "Up" indicates the robots are "above" the bag, and "down" indicates all robots are below the bag. We will add an explanatory figure.

5b. We will remove the parenthesis.  

5c.  Yes. "$\textsf{Occupied}(x_\textsf{init}) = \{s\}$" is the formal notation for the fact that all robots start at $s$. 

5d. Indeed, by "time" we mean the length of the transition sequence. We will clarify this in the exposition. This measure is a standard efficiency measure in the literature, see e.g. [5,6,7,8,9]~\cite{charrier2020complexity}. We note that in practice, long edges can be split into a sequence of shorter ones by inserting additional nodes.  


% When we mapped floor plans to graphs, we made sure edges have roughly the same physical length, splitting them when necessary and adding vertices along the way. For instance, for a corner that is not associated with a room, was still mapped to a vertex. These added vertices have a small degree and since the algorithm scales with graph size, this works quite well. Notably, when movement of the robots is coordinated, it seems hard to have edges with varying lengths, as a robot will be ``in the middle'' of edges when another one lands on a vertex. In this sense, this middle-point should be a vertex and the edge should be split.

[1] @article{almadhoun2019survey,
  title={A survey on multi-robot coverage path planning for model reconstruction and mapping},
  author={Almadhoun, Randa and Taha, Tarek and Seneviratne, Lakmal and Zweiri, Yahya},
  journal={SN Applied Sciences},
  volume={1},
  pages={1--24},
  year={2019},
  publisher={Springer}
}

[2] @article{khamis2015multi,
  title={Multi-robot task allocation: A review of the state-of-the-art},
  author={Khamis, Alaa and Hussein, Ahmed and Elmogy, Ahmed},
  journal={Cooperative robots and sensor networks 2015},
  pages={31--51},
  year={2015},
  publisher={Springer}
}

[3] @inproceedings{mathew2015optimal,
  title={Optimal path planning in cooperative heterogeneous multi-robot delivery systems},
  author={Mathew, Neil and Smith, Stephen L and Waslander, Steven L},
  booktitle={Algorithmic Foundations of Robotics XI: Selected Contributions of the Eleventh International Workshop on the Algorithmic Foundations of Robotics},
  pages={407--423},
  year={2015},
  organization={Springer}
}

[4] @article{berger2016static,
  title={Static target search path planning optimization with heterogeneous agents},
  author={Berger, Jean and Lo, Nassirou and Barkaoui, Mohamed},
  journal={Annals of Operations Research},
  volume={244},
  pages={295--312},
  year={2016},
  publisher={Springer}
}

[5] @article{fraigniaud2006collective,
  title={Collective tree exploration},
  author={Fraigniaud, Pierre and Gasieniec, Leszek and Kowalski, Dariusz R and Pelc, Andrzej},
  journal={Networks: An International Journal},
  volume={48},
  number={3},
  pages={166--177},
  year={2006},
  publisher={Wiley Online Library}
}

[6] @article{cabrera2012flooding,
  title={A flooding algorithm for multirobot exploration},
  author={Cabrera-Mora, Flavio and Xiao, Jizhong},
  journal={IEEE Transactions on Systems, Man, and Cybernetics, Part B (Cybernetics)},
  volume={42},
  number={3},
  pages={850--863},
  year={2012},
  publisher={IEEE}
}

[7] @inproceedings{sinay2017maintaining,
  title={Maintaining Communication in Multi-Robot Tree Coverage.},
  author={Sinay, Mor and Agmon, Noa and Maksimov, Oleg and Kraus, Sarit and Peleg, David},
  booktitle={IJCAI},
  pages={4515--4522},
  year={2017}
}

[8] @article{charrier2020complexity,
  title={Complexity of planning for connected agents},
  author={Charrier, Tristan and Queffelec, Arthur and Sankur, Ocan and Schwarzentruber, Fran{\c{c}}ois},
  journal={Autonomous Agents and Multi-Agent Systems},
  volume={34},
  pages={1--31},
  year={2020},
  publisher={Springer}
}
